# Supplementary material for: Differentially Private Data Release over Multiple Tables
Source: arXiv:2306.15201 source file (2023-06-27)
Supplement: Supplementary file 2 [file appendix.tex]

\appendix
\newcommand{\B}{\mathbb{J}}
\newcommand{\A}{\mathbb{F}}
\section{Missing Proof in Section~\ref{sec:intro}}
\label{appendix:single-table}

We adapt the single-table proof to our context. Let $\B$ be a table of $n$ data items over domain $\D$.  Define $\Q = \{q: \D \to [-1,+1]\}$ be the set of linear queries. Let $\A_i$ be the distribution returned by MWEM algorithm in the $i$-iteration.
Define $\ME_i = \max_q |q(\A_{i-1}) - q(\B)|$ as the maximum error over all queries in terms of $\A_{i-1}$ and $\B$. Now we are going to bound the maximum error of the MWEM algorithm:
\begin{align*}
   \max_q |q(\textrm{avg}_{i \le T} \A_i) - q(\B)|
    & = \max_q |\textrm{avg}_{i \le T} q(\A_i) - q(\B)| \\
    & \le \max_q \textrm{avg}_{i \le T} |q(\A_i) - q(\B)| \\
    & \le \textrm{avg}_{i \le T} \max_q |q(\A_i) - q(\B)|  \\
    & \le \textrm{avg}_{i \le T} \ME_i
\end{align*}
Define $\AE = 2T \cdot \frac{\widetilde{\Delta}}{\epsilon} \cdot \log |\Q|$ for $\widetilde{\Delta} = \Delta + G_{\epsilon, \delta, 1}$. Note that the sensitivity for invoking the exponential mechanism is 
\begin{align*}
    \max_{\B, \B' \textrm{are neighboring}} \max_q |q(\B) - q(\B')| \le \big||\B| -|\B'|\big| \le \Delta \le \widetilde{\Delta}
\end{align*}
and that for invoking the laplacian mechanism is
\begin{align*}
 & \max_{\B, \B' \textrm{are neighboring}} \max_q  \max_{i \in \{1,2,\cdots,T\}} |s_i(\B,q) - s_i(\B',q)| \\
 \le & \max_{\B, \B' \textrm{are neighboring}} \max_q  |q(\B) - q(\B')| \le \widetilde{\Delta}
\end{align*}
followed by the similar argument. 

\begin{lemma}
\label{lem:error}
With probability at least $1-2T/|\Q|^c$ for any $c \ge 0$, for all $1 \le i \le T$, we have:
\begin{align*}
    & |q_i(\A_{i-1}) - q_i(\B)| \ge \ME_i - (2c + 2) \times \AE\\
    & |m_i - q_i(\B)| \le c \times \AE
\end{align*}
\end{lemma}

\begin{proof}
For the first inequality, we note that the probability the exponential mechanism with parameter $\frac{\epsilon}{2T \cdot \widetilde{\Delta}}$ selects a query with quality score at least $r$ less than the optimal is bounded by 
\[\Pr[|q_i(\A_{i-1}) - q_i(\B)| < \lambda_i - (2c+2) \times \gamma] \le |\Q| \times \exp(-\frac{\epsilon \gamma}{4T \cdot \widetilde{\Delta}}) \le \frac{1}{|\Q|^c}\]
For the second inequality, we note that $|m_i - q_i(\B)|  \le c \cdot \gamma$ happens if and only if $\left|\textsf{Lap}_{\frac{2T \cdot \widetilde{\Delta}}{\epsilon}}(x)\right| \le c \cdot \gamma$ happens. By definition of the Laplace distribution, we have:
\begin{align*}
    & \Pr\left[\left|\textsf{Lap}_{\frac{2T \cdot \widetilde{\Delta}}{\epsilon}}(x)\right| > c \cdot 2T \cdot \frac{\widetilde{\Delta}}{\epsilon} \cdot \log |\Q| \right] \le \exp(-c \cdot \log |\Q|) = \frac{1}{|\Q|^c}
\end{align*}
A union bound over $2T$ events yields such a failure probability.
\end{proof}


Then, how the MW mechanism improve the approximation in each round where $q_i(\A_{i}) - q_i(\B)$ has large magnitude. To capture the improvement, we use the relative entropy function:
\begin{align*}
\Psi'_i = \frac{1}{n} \sum_{x \in \D} \B(x) \log \left(\frac{\B(x)}{\A_i(x)}\right), \ \Psi_i = \frac{n}{\hat{n}} \cdot \Psi_i 
\end{align*}
Here, we can only show that 
\begin{align*}
    \Psi_0 &= \frac{1}{\widehat{n}} \cdot \sum_{t \in \D} J(t) \log \frac{J(t)}{\F_{0}(t)}  
    \le  \frac{|\B|}{\widehat{n}} \cdot \log \frac{|\B| \cdot |\D|}{\widehat{n}} \le \log |\D|\\
    \Psi_i &= - \frac{1}{\widehat{n}} \cdot \sum_{t \in \D} \B(t) \log \frac{\F_i(t)}{\B(t)}
    \ge -\frac{1}{\widehat{n}} \sum_{t \in \D'} \F_i(t) + \frac{|\B|}{\widehat{n}} \ge -1
\end{align*}
where $\D' \subseteq \D$ such that $J(t) > 0$ for every $t \in \D'$. 

\medskip
We next consider how $\Psi$ changes in each iteration:
\begin{align*}
    \Psi_i - \Psi_{i-1} = & \frac{1}{\hat{n}} \cdot \sum_{x \in \D} \B(x) \cdot\log \left(\frac{\A_{i}(x)}{\A_{i-1}(x)}\right) \\
    =& \frac{1}{\hat{n}} \cdot q_i(\B) \cdot \eta_i -  \frac{n}{\hat{n}}\log \beta_i
\end{align*}
where 
\begin{align*}
    \eta_i &= \frac{1}{2\hat{n}} \cdot (m_i - q_i(\A_{i-1})), \\
    \beta_i &= \frac{1}{\hat{n}} \cdot \sum_{x \in \D} \exp(q_i(x) \eta_i)\A_{i-1}(x).
\end{align*}
Using the fact that $\exp(x) \le 1+x+x^2$ for $|x| \le 1$ and $|q_i(x)\eta_i| \le 1$,
\begin{align*}
    \beta_i \le & \frac{1}{\hat{n}} \cdot \sum_{x \in \D}(1+q_i(x) \eta_i + q^2_i(x) \eta^2_i) \A_{i-1}(x) \\
    \le & \frac{1}{\hat{n}} \cdot \sum_{x \in \D}(1+q_i(x) \eta_i + \eta^2_i) \A_{i-1}(x) \\
    \le & 1 + \frac{1}{\hat{n}} \cdot \eta_i q_i(\A_{i-1}) +  \eta^2_i
\end{align*}
Then, we can rewrite $\Psi_i - \Psi_{i-1}$ in the following way:
\begin{align*}
    \Psi_i - \Psi_{i-1} 
    = & \frac{1}{\hat{n}} \cdot q_i(\B) \cdot \eta_i - \log \beta_i \\
    \ge & \frac{1}{\hat{n}} \cdot q_i(\B) \cdot \eta_i - \left(\frac{1}{\hat{n}} \cdot \eta_i q_i(\A_{i-1}) +  \eta^2_i\right) \\
    %=& \frac{1}{n} \cdot \eta_i \cdot (q_i(\B) - q_i(\A_{i-1}) - \eta^2_i \\
    \ge & \eta_i \cdot \left(\frac{q_i(\B) - q_i(\A_{i-1})}{\hat{n}} - \frac{m_i - q_i(\A_{i-1})}{2\hat{n}}\right) \\
    =& \frac{m_i - q_i(\A_{i-1})}{2\hat{n}} \cdot \frac{2q_i(\B) - m_i - q_i(\A_{i-1})}{2\hat{n}} \\
    =& \left(\frac{q_i(\B) -q_i(\A_{i-1}) }{2\hat{n}}\right)^2 - \left(\frac{q_i(\B) -m_i}{2\hat{n}}\right)^2 \\
    \ge & \frac{1}{4\hat{n}^2} \cdot \left((\ME_i - 4 \AE)^2 - \AE^2 \right)
\end{align*}
where the last inequality follows the previous analysis by taking $c=1$. 
By rewritting the last inequality, we have
\begin{align*}
   \ME_i \le \sqrt{4\hat{n}^2 \cdot (\Psi_i - \Psi_{i-1}) + \AE^2} + 4 \times \AE
\end{align*}
Then,
\begin{align*}
    \textrm{avg}_{i \le T} \ME_i \le & \sqrt{4\hat{n}^2 \cdot \textrm{avg}_{i \le T} (\Psi_i - \Psi_{i-1}) + \AE^2 } + 4 \times \AE \\
    \le & 2\hat{n} \cdot \sqrt{\frac{\log |\D|}{T}} + 5 \times \AE \\
    = & O\left(\hat{n} \cdot \sqrt{\frac{\log |\D|}{T}} + \frac{T \cdot \log |\Q| \cdot \widetilde{\Delta}}{\epsilon}\right)
\end{align*}
By taking $T = \left(\frac{\widehat{n} \cdot \epsilon \cdot \sqrt{\log |\D|}}{\widetilde{\Delta} \cdot \log |\Q|}\right)^{2/3}$, we can obtain the minimized error as $O\left(\widehat{n}^{2/3} \cdot \left(\frac{\log |\Q| \cdot \widetilde{\Delta}\cdot \log |\D|)}{\epsilon}\right)^{1/3} \right)$.bIn $(\epsilon, \delta)$-DP, this error can be generalized as (omitting the fact of $\left(\frac{\log |\Q| \cdot \log \frac{1}{\delta} \cdot \log^{\frac{1}{2}} |\D|)}{\epsilon}\right)^{1/2}$):
\[O\left(\sqrt{\widehat{n}} \cdot \sqrt{\widetilde{\Delta}} \right) = O\left(\sqrt{|\B|} \cdot \sqrt{\widetilde{\Delta}} + \widetilde{\Delta}\right) \]

%\pasin{I think one way to get a similar result as above is the following: if in our new version, we can move up to $\Delta$ $x$'s, then we may apply the old (sensitivity-1) algorithm but with $\epsilon = \epsilon/\Delta$; group-DP then ensures that the algorithm is $\epsilon$-DP under the new neighboring notion. This gives similar bound as above.}


%\xiao{What's the optimal choice of $T$ in $(\epsilon',\delta)$-DP?} 
%\[T = \frac{n \cdot \epsilon' \cdot \sqrt{\log \D}}{\log |\Q| \cdot \log \frac{1}{\delta}}\]

\section{Missing Proofs in Section~\ref{sec:join-as-one}}
\label{appendix:join-as-one}

\begin{lemma}
\label{lem:up-2table-join-size}
    For any pair of neighboring instance $\I,\I'$, let $J,J'$be the join results of $\I, \I'$ respectively. Then, $\big||J|-|J'|\big| \le \widetilde{\Delta}$.
\end{lemma}

Lemma~\ref{lem:up-2table-join-size} directly follows the definition of $LS_\countsize(\I)$ and the non-negative property of $\textsf{STGeom}$.

 
\begin{proof}[Proof of Lemma~\ref{lem:two-table-DP}]
    Consider two neighboring database $\I = (R_1, R_2)$ and $\I'=(R'_1, R'_2)$. We first prove $\widehat{n} \sim_{(2\epsilon, 2\delta)} \widehat{n'}$. Let $\Delta, \Delta'$ be the local sensitivity of $\I,\I'$ respectively. It can be easily checked that $|\Delta - \Delta'| \le 1$.  Let $\widetilde{\Delta}, \widetilde{\Delta'}$ be the random variables by adding random noises from $\textsf{STGeom}_{\epsilon, \delta, 1}$ to $\Delta, \Delta'$ separately. Let $\textsf{supp}\left(\widetilde{\Delta}\right),  \textsf{supp}\left(\widetilde{\Delta'}\right)$ be the support of $\widetilde{\Delta}, \widetilde{\Delta'}$ separately. 
    From \textsf{STGeom}, we observe:
    \begin{equation}
        \label{eq:proof-2table}
        \Delta + \textsf{STGeom}_{\epsilon, \delta, 1}(x) \sim_{(\epsilon, \delta)} \Delta' + \textsf{STGeom}_{\epsilon, \delta, 1}(x) 
    \end{equation}
    since $|\Delta - \Delta'| =1$, hence $\widetilde{\Delta} \sim_{(\epsilon, \delta)} \widetilde{\Delta'}$. We next note that for any $\widehat{\Delta} \in \textsf{supp}\left(\widetilde{\Delta}\right) \cup \textsf{supp}\left(\widetilde{\Delta'}\right)$, the following holds:
    \begin{align*}
        |J| + \textsf{STGeom}_{\epsilon, \delta, \widehat{\Delta}}(x) \sim_{(\epsilon, \delta)} |J'| + \textsf{STGeom}_{\epsilon, \delta, \widehat{\Delta}}
    \end{align*}
    since $\big||J| - |J'|\big|\le \widetilde{\Delta}$. From the sequential composition rule~\cite{dwork2006calibrating, dwork2006our}, we conclude that $\widehat{n} \sim_{(2\epsilon, 2\delta)} \widehat{n}'$.

    We next turn to line 6. Let $\F, \F'$ be the synthetic data generated for $(R_1, R_2), (R'_1, R'_2)$ separately. The single-table algorithm starts with a uniform distribution with $\F_0(x) = \frac{\widehat{n}}{|\D|}$ for $(R_1, R_2)$, and $\F'_0(x) = \frac{\widehat{n}'}{|\D|}$ for $(R'_1, R'_2)$. Implied by the analysis above, the initial state satisfies $(2\epsilon, 2 \delta)$-DP, i.e., $\F_0 \sim_{(2\epsilon, 2 \delta)} \F'_0$. 

    We finally come to line 6-9, with $T$ invocations to the EM Mechanism and Laplace mechanism. For exponential mechanism, let $q_j, q_{j'}$ be the query selected after line 7. For Laplace mechanism, let $m_i, m'_i$ be the resulted value after line 9 for $(R_1, R_2), (R'_1, R'_2)$ respectively. From previous, we already have (\ref{eq:proof-2table}).
We next note two facts for any $\widehat{\Delta} \in \textsf{supp}\left(\widetilde{\Delta}\right) \cup \textsf{supp}\left(\widetilde{\Delta'}\right)$: 
\begin{itemize}[leftmargin=*]
    \item $j \sim_{(\epsilon, \delta)} j'$ since $s_i(J, q) - s_i(J', q) \le |q(J) - q(J')| \le \big||J| - |J'|\big| \le \widehat{\Delta}$ holds for every query $q$,
\end{itemize}
\begin{align*}
    q_i(J) + \textsf{STGeom}_{\frac{\epsilon}{2T}, \delta, \widehat{\Delta}}(x)  \sim_{(\frac{\epsilon}{2T}, \delta)}() q_i(J') + \textsf{STGeom}_{\frac{\epsilon}{2T}, \delta, \widehat{\Delta}}(x)
\end{align*}
since $\big|q_i(J) - q(J')\big| \le |J - J'| \le \Delta \le \widehat{\Delta}$. Summing over $T$ iterations, it yields
$(\epsilon,\delta)$-DP. Thus,
Algorithm~\ref{alg:two-table} preserves $(3\epsilon, 3\delta)$-DP. 
\end{proof}

\begin{proof}[Proof of Lemma~\ref{lem:multi-table-DP}]
For any pair of neighboring instance $\I,\I'$, we note that $SS^\beta_\countsize(\I) \le e^{\beta} \cdot SS^\beta_\countsize(\I')$ always holds. Let $\widetilde{\Delta}, \widetilde{\Delta}'$ be the updated value after line 3 for $\I,\I'$ respectively. It can showed that with probability at least $1- \delta$, $|\textsf{Lap}_1(x)| < \ln \frac{2}{\delta}$, then $\frac{\beta}{\epsilon} \textsf{Lap}_1(x) + \frac{1}{2}\in [0,1]$, and therefore $\widetilde{\Delta} \in [SS^\beta_\countsize(\I), SS^\beta_\countsize(\I) \cdot e]$. For any $y \in [SS^\beta_\countsize(\I),+\infty)$, we have 
\begin{align*}
    \frac{\Pr[\widetilde{\Delta}  = y]}{\Pr[\widetilde{\Delta}' = y]} = \exp\left(\frac{\epsilon}{\beta} \cdot \log \frac{SS_\countsize(\I)}{SS_\countsize(\I')}\right) \le \exp(\epsilon)
\end{align*}
thus, $\widetilde{\Delta} \sim_{(\sigma, \delta)} \widetilde{\Delta}'$. Then, for any $\widehat{\Delta} \in \textsf{supp}\left(\widetilde{\Delta}\right) \cup \textsf{supp}\left(\widetilde{\Delta}'\right)$, we know that
\[|J| + \textsf{STGeom}_{\epsilon, \delta, \widehat{\Delta}}(x) \sim_{(\epsilon, \delta)} |J'| + \textsf{STGeom}_{\epsilon, \delta, \widehat{\Delta}}(x) \]
since $\big||J| - |J'| \big| \le LS_\countsize(\I) \le SS_\countsize(\I) \le \widehat{\Delta}$. Let $\widehat{n}, \widehat{n}'$ be the resulted value after line 5 for $\I, \I'$ respectively. Then, $\widehat{n}\sim_{(2\epsilon, 2\delta)} \widehat{n}'$.

We next turn to line 6. Let $\F, \F'$ be the synthetic data generated for $\I, \I'$ separately. The single-table algorithm starts with a uniform distribution with $\F_0(x) = \frac{\widehat{n}}{|\D|}$ for $(R_1, R_2)$, and $\F'_0(x) = \frac{\widehat{n}'}{|\D|}$ for $(R'_1, R'_2)$. Implied by the analysis above, the initial state satisfies $(2\epsilon, 2 \delta)$-DP, i.e., $\F_0 \sim_{(2\epsilon, 2 \delta)} \F'_0$. 


We finally come to line 7-10, with $T$ invocations to the
EM Mechanism and Laplace mechanism. For exponential mechanism, let $q_j, q_{j'}$ be the query selected after line 7. For Laplace mechanism, let $m_i, m'_i$ be the resulted value after line 9 for $\I, \I'$ respectively. As previous, we already showed that $\displaystyle{\widetilde{\Delta} \sim_{(\epsilon, \delta)} \widetilde{\Delta}'}$.
We next note two facts for any $\widehat{\Delta} \in \textsf{supp}\left(\widetilde{\Delta}\right) \cup \textsf{supp}\left(\widetilde{\Delta'}\right)$: 
\begin{itemize}[leftmargin=*]
    \item $j \sim_{(\epsilon, \delta)} j'$;
    \item $q_i(J) + \textsf{STGeom}_{\frac{\epsilon}{2T}, \delta, \widehat{\Delta}}(x) \sim_{(\frac{\epsilon}{2T}, \delta)} q_i(J') + \textsf{STGeom}_{\frac{\epsilon}{2T}, \delta, \widehat{\Delta}}(x)$
\end{itemize}
The first one follows the fact that $s_i(J, q) - s_i(J', q) \le |q(J) - q(J')| \le \big||J| - |J'|\big| \le LS_\countsize(\I) \le SS_\countsize(\I) \le \widehat{\Delta}$ holds for every query $q$. The second one follows from the fact that $\big|q_i(J) - q(J')\big| \le |J - J'| \le \Delta \le \widehat{\Delta}$.
Summing over $T$ iterations, it results
in $(\epsilon,\delta)$-DP. Thus,
Algorithm~\ref{alg:two-table} preserves $(3\epsilon, 3\delta)$-DP. 
\end{proof}

\begin{proof}[Proof of Theorem~\ref{the:lb-multi-table}]
Set $n= \frac{\OUT}{\Delta}$ and $\D = (\{0,1\}^d)^n$. From Theorem~\ref{the:lb-single-table}, let $\Q_\textsf{one}$ be the set of queries on which any $(\epsilon, \delta)$-differentially private algorithm that takes as input a single-table database $T \in \D$ and output an approximate answer to each query in $\Q_\textsf{one}$ within $\ell_\infty$-error $\alpha$ requires that $\alpha \ge \widetilde{\Omega}\left(\sqrt{n} \cdot (\frac{\sqrt{d} \log |\Q_\textsf{one}|}{\epsilon})^{\frac{1}{2}}\right)$.
For an arbitrary single-table database $T \in \D$, we construct
a multi-table instance $\I$ for $\mathcal{H}$ of input size $m$, join size $\OUT$, and local sensitivity $\Delta$ as follows:
Without loss of generality, we pick $\x_1$ as the anchor relation to encode $T$. 
\begin{itemize}[leftmargin=*]
    \item Set $\dom(x) = \D$ if $x \in \x_1$, and $\dom(x) = \mathbb{Z}$ otherwise; 
    \item There are $\Delta^{\frac{1}{k}}$ distinct values in $\dom(x)$ for $x \notin \x_1$, where $k = \left|\bigcup_{i \in [m]} \x_i - \x_1\right|$;
    \item For each data record $y \in T$, we add a tuple $(y,y,\cdots, y)$ in $R_1$;  
    \item Tuples in $R_i$ for $i\ge 2$ form a Cartesian product of size $\Delta^{\frac{|\x_i|}{k}}$ over all attributes in $\x_i$;
\end{itemize}
It can be easily checked that $\I \in \mathbb{I}(\OUT,\Delta)$. 
From $\Q_\textsf{one}$, we construct a set of queries over $\I$ as $\Q_\textsf{hier}$. For each query $q \in \Q_\textsf{one}$, we construct another query $q'=(q_1,q_2, \cdots, q_m)$ as follows:
\begin{itemize}[leftmargin=*]
    \item $q_1: \D_1 \to [0,1]$ such that $q_1(t) = q(y)$ if and only if $\pi_x t = y$ for any $x \in \dom(x_1)$;
    \item $q_i: \D_i \to \{+1\}$ over $\D_i$ for $i \ge 2$.
\end{itemize}
We also add the counting query $q' = (q_1,q_2, \cdots, q_m)$ with $q_i: \D_i \to \{+1\}$ for any $i \in [m]$ to $\Q_\textsf{two}$.

It suffices to show that if there is a $(\epsilon, \delta)$-differentially private algorithm that takes any multi-table instance in $\mathbb{I}(\OUT, \Delta)$ and outputs an approximate answer to each query in $\Q_\textsf{hier}$ within error $\alpha$, then there is a $(\epsilon, \delta)$-differentially private algorithm that takes any single-table instance $T \in \D$ and outputs an approximate answer to each query in $\Q_\textsf{one}$ within error $\frac{\alpha}{\Delta}$. The remaining argument exactly follows that of two-table case.
\end{proof}


%\subsection{Uniformize Star Join}
%Let's start with the star join: $R_1(A_1,B)\Join R_2(A_2,B) \Join \cdots \Join R_m(A_m,B)$, which is also the simplest class of hierarchical joins.  Note that there is a single join attribute $B$ in this query. Similar to the two-table case, we partition the instance $\I$ by join values into multiple sub-instances, such that join values with similar degrees will fall into the same sub-instance. 
%Note that the maximum degree of a join value in any relation is at most $n$. After adding a non-negative noise $\textsf{STGeom}_{\epsilon, \delta, 1}(x)$, the maximum possible noisy degree is $n+ \lambda$. We partition $[0,n+ \lambda]$ into $\ell= \lceil \log_2 (\frac{n}{\lambda} + 1)\rceil$ disjoint intervals, where the $i$-th interval is defined as $(\lambda \cdot 2^{i-1}, \lambda \cdot  2^i]$ for $i \ge 1$, and $(0, \lambda]$ for $i=0$. We note that each $\sigma \in [\ell] \times [\ell] \times \cdots [\ell]$ defines a degree characterization. More specifically, the set of join values whose degree in $R_i$ falls into the $\sigma(i)$-th bucket for each $i\in [m]$ is denoted as $B^{\sigma}$.
%From each $\sigma$, we identify tuples in $R_j$ whose join value falls into $B^{\sigma}$ as $R^{\sigma}_j$. Hence, we obtain a sub-instance $(R^{\sigma}_1, R^{\sigma}_2, \cdots, R^{\sigma}_m)$ corresponding to $\sigma$, and return the sub-instances for all $\sigma$'s. 
%
\begin{algorithm}
\caption{{\sc Uniformize-Star}$(\I = \{R_1, R_2, \cdots, R_m\})$}
\label{alg:uniformization}


\lForEach{$i \in [m]$}{$\ell_i \gets \lceil \log (\frac{n}{\lambda} + 1)\rceil$}
$B^{\sigma} \gets \emptyset$ for each $\sigma \in [\ell]^m$\;
\ForEach{$b \in B$}{
    \ForEach{$i \in [m]$}{
        $\displaystyle{\deg_i(B,b) = \degg_i(B,b) + \textsf{STGeom}_{\epsilon, \delta, 1}(x)}$\;
       }
       $\sigma \gets \left \langle \max\left\{0, \left\lceil\log \frac{1}{\lambda} \cdot \deg_i(B,b) \right\rceil \right\}: i \in [m]\right\rangle$\;
       $B^{\sigma} \gets B^{\sigma} \cup \{b\}$\;
}
\ForEach{$\sigma \in [\ell]^m$}{
    \ForEach{$i \in [m]$}{
        $R^{\sigma}_i\gets \{R_i(t): t \in \D_i, \pi_B t \in B^{\sigma}\}$\;
    }
}
\Return $\bigcup_{\sigma \in [\ell]^m}\left\{(R^{\sigma}_1, R^{\sigma}_2, \cdots, R^{\sigma}_m)\right\}$\;
\end{algorithm}


%\subsection{Uniformize Line-3 Join using Elastic Sensitivity}
%
%\paragraph{Uniformization.} The uniformization over line-3 join becomes unclear, since the residual sensitivity display a more complicated form. But, we can apply the similar strategy as two-table case on $B,C$ separatel.
%
%We partition $(0, n+\lambda]$ into $\ell = \lceil \log(\frac{n}{\lambda}+1)\rceil$ disjoint intervals, where the $i$-th interval is defined as $(\lambda \cdot 2^{i-1}, \lambda \cdot 2^i]$ for $i \in [\ell]$. Then the join values from $B$ whose noisy degree in $R_1$ falls into the $i$-interval and noisy degree in $R_2$ falls into the $j$-interval is denoted as $B^{(ij)}$. 
%
%\paragraph{Step 2: Instance partition and Invoke single-table independently.}Now consider each combination of $\sigma = (i,j,k,h)\in [\ell_1] \times [\ell_2] \times [\ell_3] \times [\ell_4]$. For simplicity, we denote $B^{(\sigma(1), \sigma(2))}$ as $B^{\sigma}$, and $C^{(\sigma(3), \sigma(4))}$ as $C^{\sigma}$. The corresponding sub-instance defined by $\sigma$ is noted as $\I^{\sigma}$, consisting of
%\begin{align*}
%    R^{\sigma}_1 =& \left\{R_1(t): t \in \D_1, \pi_{B} t \in B^{\sigma}\right\} \\
%    R^{\sigma}_2 =& \left\{R_2(t): t \in \D_2, \pi_{B} t \in B^{\sigma}, \pi_{C} t \in C^{\sigma}\right\} \\
%    R^{\sigma}_3 =& \left\{R_3(t): t \in \D_3, \pi_{C} t \in C^{\sigma} \right\}
%\end{align*}
%We then invoke {\sc MultiTable} algorithm to release a synthetic dataset $\F^\sigma$ for $\I^\sigma$. At last, we return the union of all synthetic dataset.


%\paragraph{Issue.} Recall that our target is to get a tight bounded for local sensitivity over each sub-instance as much as possible.  In terms of $\countsize\left(\I^{\sigma}\right)$, we mention the following observations on different notions of sensitivity. First, the \xiao{elastic sensitivity} is exactly captured by $\sigma$, which is defined as  \[ES_\countsize(\I^{\sigma}) = \max \left\{2^{\sigma(1) + \sigma(4)}, 2^{\sigma(1) + \sigma(3)}, 2^{\sigma(2) + \sigma(4)} \right\}.\] Secondly, the local sensitivity (as well as smooth sensitivity) is \begin{displaymath}  LS_\countsize(\I^{\sigma}) = \max \left\{ \begin{array}{ll} \displaystyle{2^{\sigma(1) + \sigma(4)}}&\\ \displaystyle{2^{\sigma(1)} \max_{c \in C^{\sigma}} \sum_{b \in B^{\sigma}} R^\sigma_2(b,c)}&\\ \displaystyle{2^{\sigma(4)} \max_{b \in B^{\sigma}} \sum_{c \in C^{\sigma}} R^\sigma_2(b,c) }& \end{array} \right.  \end{displaymath} which does not have a tight bound only using $\sigma$. For simplicity, we assume all $\deg_1(B,b)$'s and $\deg_3(C,c)$'s are the same for all values $b \in \dom(B)$ and $c \in \dom(C)$.

\subsubsection{Missing Proofs for the Lower Bound}

\begin{proof}[Proof of \Cref{the:lb-two-table-1}]
    Let $\Q = \{\countsize\}$. Let $\I, \I'$ be a pair of neighboring instances $\I,\I' \in \bbI(\Delta)$ such that $|\countsize(\I) - \countsize(\I')| \geq \Omega(\Delta)$.

    Suppose for the sake of contradiction that there is an $(\epsilon, \delta)$-DP algorithm $\cA$ that achieves an error $\alpha < |\countsize(\I) - \countsize(\I')| / 2$ with probability at least 0.99. Let $\widetilde{\countsize}(\I), \widetilde{\countsize}(\I')$ be the results released for join sizes of $\I, \I'$ respectively. Then, as $\cA$ preserves $(\epsilon, \delta)$-DP, it must be that
    \begin{align*}
        0.99 &\leq \Pr\left(\widetilde{\countsize}(\I) \in [\countsize(\I)-\alpha, \countsize(\I) + \alpha] \right) \\
        &\le e^\epsilon \cdot \Pr\left(\widetilde{\countsize}(\I') \in [\countsize(\I)-\alpha, \countsize(\I) + \alpha]\right) + \delta \\
        &< e^\epsilon \cdot \left(1 - \Pr\left(\widetilde{\countsize}(\I') \in [\countsize(\I')-\alpha, \countsize(\I') + \alpha]\right)\right) + \delta \\
        &\leq e^\eps \cdot 0.1 + \delta < 0.99,
    \end{align*}
    a contradiction.
\end{proof}



\subsection{Missing Proofs in Section~\ref{sec:uniformization}}
\label{appendix:uniformization}

\begin{example}
\label{exp:1}
    Consider an example that $|J^{i}| = \frac{|J|}{\ell}$ for each $i \in [\ell]$. Algorithm~\ref{alg:two-table} achieves an error as
    $\alpha = O\left(\sqrt{|J|} \cdot \sqrt{\Delta} + \Delta\right)$, while Algorithm~\ref{alg:uniformization} achieves an error as \[\alpha = \sum_{i\in [\ell]} \sqrt{\frac{|J|}{\ell}} \cdot \sqrt{2}^{i} + \sum_{i\in [\ell]} \Delta_i = \sqrt{\frac{|J|}{\ell}} \cdot \sqrt{2}^{\ell+1} + \Delta = O\left(\sqrt{\frac{|J|}{\ell}} \cdot \sqrt{\Delta} + \Delta \right)\]
    where we can save a factor of $\sqrt{\ell} = O(\sqrt{\log n})$. 
\end{example}

\begin{example}
\label{exp:2}
    Consider an example that $|J^{i}| \cdot \Delta_i = \Delta^2$ for each $i \in [\ell]$, by setting $|B^{i}| = 4^{\ell-i}$ and $|J^{i}| =4^{\ell-i} \cdot 2^i$. The total number of join results is $|J| = \sum_{i \in [\ell]} |J^{i}| = \sum_{i \in [\ell]} 4^{\ell-\frac{i}{2}} \le 4^\ell = \Delta^2$.
    By setting $\Delta =\sqrt{n}/\log n$, the total number of tuples is at most 
    $\sum_{i \in [\ell]} 2^i \cdot 4^{\ell-i} = 4^\ell \cdot \sum_{i \in [\ell]} 4^{-i} \le \Delta^2 = n$. Algorithm~\ref{alg:two-table} achieves an error as
    $\alpha =O(\Delta \cdot \sqrt{\Delta})$, while Algorithm~\ref{alg:uniformization} achieves an error as
    \[\alpha = \sum_{i\in [\ell]} \sqrt{4^{\ell-i} \cdot 2^i} \cdot \sqrt{2^i} + \Delta = 2^{\ell} \cdot \ell+ \Delta  = O(\Delta \cdot \log n)\]
    where we can save a factor of $O(\sqrt{\Delta}) = O(n^{1/4})$.
\end{example}

\begin{proof}[Proof of Lemma~\ref{lem:partition-2table-DP}]
    Consider two neighboring instances $\I = (R_1, R_2)$ and $\I' = (R'_1, R'_2)$. Let $\sigma, \sigma':\dom(B) \to [\ell]$ be the partitions of $\dom(B)$ for $\I,\I'$ respectively. By definition, $\sigma(b) = i$ if and only if $b \in B^{i}$; $\sigma'$ is defined similarly. Note that $|\degg_i(B, b) - \degg'_i(B,b)|\le 1$ holds for any $i\in\{1,2\}$ and $b \in \dom(B)$. Hence, $\sigma(b) \sim_{(\epsilon, \delta)} \sigma'(b)$. As the degrees for different $b$'s are calculated on disjoint parts of input data, then $\sigma \sim_{(\epsilon, \delta)} \sigma'$ from the parallel composition rule. 
    
    Let $\F^{i},\F'^{i}$ be the synthetic dataset generated for $(R^i_1, R^i_2), (R'^i_1, R'^i_2)$ respectively. Implied by Lemma~\ref{lem:two-table-DP}, $\F^{i} \sim_{(3\epsilon, 3\delta)} \F'^{i}$ for each $i \in [\ell]$.
    Note that $\{(R^{i}_1, R^{i}_2):i\in [\ell]\}$ forms a disjoint partition of $(R_1, R_2)$. By the parallel composition rule, $\bigcup_{i \in [\ell]} \F^{i} \sim_{(3\epsilon, 3\delta)} \bigcup_{i \in [\ell]} \F'^{i}$. Putting everything together, we conclude that Algorithm~\ref{alg:uniformization} preserves $(4\epsilon, 4\delta)$-DP implied by the sequential composition rule.
\end{proof}


\begin{proof}[Proof of Theorem~\ref{the:up-2table-uniformize}]
Given an input instance $\I$ over the two-table query, let $\pi_1 = \left\{B^0_1, B^1_1, \cdots, B_1^{\lceil \log (\frac{n}{\lambda}+1)\rceil}\right\}$, be a fixed partition of $\dom(B)$, such that $b \in B^i_1$ if and only of \[\max\{\degg_1(B,b), \degg_2(B,b)\} \in  (\lambda \cdot 2^{i-1}, \lambda \cdot 2^{i}].\] Let $\pi_2 = \left\{B^0_2, B^1_2, \cdots, B_2^{\lceil \log (\frac{n}{\lambda}+1)\rceil}\right\}$ be a random partition of $\dom(B)$ by Algorithm~\ref{alg:partition-2table}. Note that $b \in B^i_2$ happens only if 
\[\max\{\degg_1(B,b), \degg_2(B,b)\} \in (\lambda \cdot 2^{i-1} - \lambda, \lambda \cdot 2^{i}].\]
It is easy to see that $B^{i+1}_1\subseteq B^{i}_2 \cup B^{i+1}_2$. For simplicity, we denote the number of join results participated by values in $B^{i}_1 \cap B^{i}_2$ as $x_i$ and the number of join results participated by values in $B^{i}_1 - B^{i}_2$ as $y_i$. Then the cost of Algorithm~\ref{alg:uniformization} under partition $\pi_2$ is 
\begin{align*}
    & \sum_{i \in [\lceil \log (\frac{n}{\lambda}+1)\rceil]}\sqrt{x_i + y_{i-1}} \cdot \sqrt{\lambda \cdot 2^{i}} \\
    \le& \sqrt{\lambda} \cdot \sum_{i \in [\lceil \log (\frac{n}{\lambda}+1)\rceil]} (\sqrt{x_i} + \sqrt{y_{i-1}}) \cdot \sqrt{2^{i}} \\
    \le & \sqrt{\lambda} \cdot \left(\sum_{i \in [\lceil \log (\frac{n}{\lambda}+1)\rceil]} \sqrt{x_i} \cdot \sqrt{2^{i}} + \sum_{i \in \lceil \log \frac{(\frac{n}{\lambda} + 1)}{\lambda}\rceil}  \sqrt{y_{i-1}} \cdot \sqrt{2^{i}}\right) \\
    \le& \sqrt{2} \cdot \sqrt{\lambda} \cdot \left(\sum_{i \in [\lceil \log (\frac{n}{\lambda}+1)\rceil]} \sqrt{x_i} \cdot \sqrt{2^{i}} + \sum_{i \in \lceil \log \frac{(\frac{n}{\lambda} + 1)}{\lambda}\rceil}  \sqrt{y_{i-1}} \cdot \sqrt{2^{i-1}}\right) \\
    =& \sqrt{2} \cdot \sqrt{\lambda} \cdot \left( \sum_{i \in [\lceil \log (\frac{n}{\lambda}+1)\rceil]} (\sqrt{x_i} + \sqrt{y_{i}} ) \cdot \sqrt{2^{i}} \right)\\
    \le & \sum_{i \in [\lceil \log (\frac{n}{\lambda}+1)\rceil]} \sqrt{x_i + y_i} \cdot \sqrt{2^{i} \cdot \lambda} 
\end{align*}
thus can be bounded by the cost of $\mathcal{A}$ under the fixed uniform partition of $\dom(B)$.
\end{proof}



\begin{proof}[Proof of Theorem~\ref{the:lb-instance-optimality-2table}]
    Let $\mathbb{I}(\OUT_i, i)$ be the set of two-table instances with output size $\OUT_i$ and every join value has maximum degree falling into $(\lambda \cdot 2^{i-1}, \lambda \cdot 2^i]$.
    Our proof consists of two steps: 
    \begin{itemize}[leftmargin=*]
        \item {\bf Step (1):} There exists a family of queries $\Q_i$ such that any $(\epsilon,\delta)$-algorithm that takes as input an instance from $\mathbb{I}(\OUT_i, i)$ and outputs an approximate answer to each query in $\Q_i$ within error $\alpha^{i}$ must require $\displaystyle{\alpha_i \ge \Omega\left(\sqrt{\OUT_i} \cdot\sqrt{2^i \cdot \lambda}\right)}$.
        \item {\bf Step (2):} There exists a family of queries $\Q$ such that any $(\epsilon,\delta)$-algorithm that takes as input an instance $\I(\overrightarrow{\OUT})$ and outputs an approximate answer to each query in $\Q$ within error $\alpha$ must require
        $\displaystyle{\alpha \ge \Omega\left(\max_i \sqrt{\OUT_i} \cdot \sqrt{2^i \cdot \lambda}\right)}$.
    \end{itemize}
    
    Let's first focus on {\bf step (1)} with arbitrary $i \in [\lceil \log (\frac{n}{\lambda}) \rceil]$.
    Let $n_i$ be an arbitrary integer such that $n_i \cdot \lambda \cdot 2^{i-1} \le \OUT_i \le n_i \cdot \lambda \cdot 2^i$ holds. From Theorem~\ref{the:lb-single-table}, let $\Q^i_\textsf{one}$ be the set of hard queries on which any $(\epsilon,\delta)$-differentially private algorithm takes as input any single table $T^i \in (\{0,1\}^d)^{n_i}$, and outputs an approximate answer to each query in $\Q^i_\textsf{one}$ within error $\alpha$ must require $\alpha \ge \widetilde{\Omega}\left(\sqrt{n_i} \cdot (\frac{\sqrt{d} \cdot \log |\Q^i_\textsf{one}|}{\epsilon})^\frac{1}{2}\right)$. For an arbitrary single table $T^i \in (\{0,1\}^d)^{n_i}$, we can construct a two-table instance $(R^i_1, R^i_2)$ as follows:
    \begin{itemize}[leftmargin=*]
    \item Set $\dom(A) = \D$, $\dom(B) = \mathbb{Z}$ and $\dom(C) = \mathbb{Z}$;
    \item Set $\D_1 = \dom(A) \times \dom(B)$ and $\D_2 = \dom(B) \times \dom(C)$;
    \item Tuples in $R^i_1$ form a Cartesian product of size $n_i \times 1$ over $\dom(A) \times \dom(B)$;
    \item Tuples in $R^i_2$ form a Cartesian product of sizes $1 \times \frac{\OUT_i}{n_i}$ over $\dom(B) \times \dom(C)$;
    \item For each of the $n$ records in $T^i$, say $x$, we add a tuple $t \in R_1$ and set $\pi_A t = x$. 
\end{itemize}
It can be easily checked that $\I \in \mathbb{I}(\OUT_i,i)$. From Theorem~\ref{the:lb-single-table}, let $\Q^i_\textsf{two}$ be the set of all linear queries over $\D^i_1 \times \D^i_2$. For each query $q \in \Q^i_\textsf{one}$, we construct another query $q'=(q_1,q_2) \in \Q^i_\textsf{two}$ such that:
    \begin{itemize}[leftmargin=*]
        \item $q_1: \D^i_1 \to [0,1]$ such that $q_1(t) = q(x)$ if and only if $\pi_A t =x$;
        \item $q_2: \D^i_2 \to \{+1\}$.
    \end{itemize}
    We borrow the similar argument from Theorem~\ref{the:lb-two-table}, showing that an $(\epsilon, \delta)$-algorithm that takes a two-table instance in $\mathbb{I}(\OUT_i, i)$ and outputs an approximate answer to each query in $\Q^i_\textsf{two}$ within error $\alpha$, there exists an $(\epsilon, \delta)$-algorithm that takes an arbitrary single table $T_i \in (\{0,1\})^{n_i}$, and outputs an approximate answer to each query in $\Q^i_\textsf{one}$ within error $\frac{\alpha^i}{\lambda \cdot 2^i}$. As $\frac{\alpha^i}{\lambda \cdot 2^i} \ge \sqrt{n_i}$, $\alpha^i \ge \sqrt{\OUT_i} \cdot \sqrt{2^i} \cdot \sqrt{\lambda}$.
    
    \paragraph{Step (2).} From Theorem~\ref{the:lb-single-table}, let $\Q_\textsf{two}$ be the family of linear queries over $\D_1 \times \D_2$, such that $\displaystyle{\Q_\textsf{two} = \left\{\cup_{i \in [m]} q_i: q_i \in \Q^{i}_\textsf{two}, \forall i \in [\lceil \log n \rceil]\right\}}$. Consider an arbitrary $(\epsilon, \delta)$-differentially private algorithm $\mathcal{A}$ takes as input in $\mathbb{I}(\overrightarrow{\OUT})$ and outputs an approximate answer to each query in $\Q_\textsf{two}$ within error $\alpha$. If $\alpha \le \max_i \sqrt{\OUT_i} \cdot \sqrt{2^i \cdot \lambda}$, there must exist an $(\epsilon, \delta)$-differentially private algorithm that takes an input any instance from $\mathbb{I}(\overrightarrow{\OUT})$ and output an approximate answer to each query in $\Q^i_\textsf{two}$, for some $i$, contradicting to {\bf Step (1)}.
\end{proof}

    In the attribute tree $\mathcal{T}$, if there exists an attribute with only one child, say $u$ with child $v$, we know that $u,v$ always appear together in all relations, then they can be simply considered as one ``combined'' attribute. Hence, it is safe to assume that every non-leaf attribute has at least two children in $\mathcal{T}$.  

\begin{proof}[Proof of Lemma~\ref{lem:partition-hierarchical}]
     We will prove the first two properties by induction. In the base case when $\mathbb{I}$ only contains one instance, these two properties hold trivially. 
     Consider an arbitrary iteration of while-loop in Algorithm~\ref{alg:uniformize-hierarchical}. By hypothesis, all sub-instances in $\mathbb{I}$ have disjoint join results, and the union of join results of all sub-instances in $\mathbb{I}$ is $\Join_{i\in [m]} R_i$. Then, it suffices to show that {\sc PartitionByAttr}$(\I, x)$ generates a partition of $\I$ as 
     \[\left\{\I^i = \left( \bigcup_{j \in E_x} R^i_j \right) \cup 
     \left( \bigcup_{j \notin E_x} R_j \right): i \in \left[\left\lceil \log \left(\frac{n}{\lambda} + 1\right) \right\rceil\right]\right\},\] 
     such that all $\I^i$'s have disjoint join results, and the union of join results of all $\I^i$'s is the join result of $\I$. 
     
     Consider an arbitrary join result $t = (t_1, t_2, \cdots, t_m)$ of $\I$, where $t_j$ is projection of $t$ onto $\x_j$. For any $j \notin E_x$, $t_j \in R_j$. Let $\vec{y} \in \dom(\y)$ be the tuple such that $\pi_{\y} t_j = \vec{y}$ holds for every  $j \in E_x$. Denote $i^* = \lceil \log \frac{1}{\lambda} \cdot \deg_{E_x}(\y, \vec{y})\rceil$. Then, for any $j \in E_x$, $t_j \in R^{i}_j$ if and only if $i = i^*$ by line 9. Thus, $t \in \left(\Join_{j \in E_x} R^{i^*}_j \right) \Join \left(\Join_{j \notin E_x} R_j\right)$, but $t \notin \left(\Join_{j \in E_x} R^{i}_j \right) \Join \left(\Join_{j \notin E_x} R_j\right)$ for any $i \neq i^*$.
     
     For the third property, we actually show that each input tuple $t \in R_i$ appears in $O(\log^{c} (\frac{n}{\lambda} + 1))$ sub-instances, where $c = \sum_{x \in \x} |E_x|$ is the total number of appearance of join attributes in all relations. In an invocation of {\sc PartitionHier}$(\I,x)$, tuple $t \in R_i$ appears in $O\left(\log (\frac{n}{\lambda} + 1) \right)$ sub-instances if $i \notin E_x$, and only one sub-instance otherwise. Overall, the procedure {\sc PartitionByAttr} will be invoked on every non-leaf attribute in $\mathcal{T}$, thus
     every input tuple $t \in R_i$ appears in 
     $O\left(\prod_{x \in \x} \log (\frac{n}{\lambda} + 1)\right) =O\left(  \log^{|\x|} (\frac{n}{\lambda} + 1) \right)$ sub-instances.
     
    At last, we first show each sub-instance corresponds to a degree characterization. Let's focus on an arbitrary single relation $\x_j$ in Algorithm~\ref{alg:uniformize-hierarchical}, which is partitioned by attributes lying on the path corresponding to $\x_j$ in $\mathcal{T}$ in a bottom-up way, say $\langle x_1, x_2, \cdots, x_k (=r)\rangle$.  When {\sc PartitionByAttr}$(\I,x_1)$ is invoked, the sub-instance $\I^i  = \{R^i_j: j \in E_{x_1}\} \cup \{R_j: j \notin E_{x_1}\}$ must have $\sigma(E_{x_1}, \y)=i$ with
    \[\deg^{\I^i}_{E_{x_1}}(\y, \vec{y}) \in \left(2^{\sigma(E_{x_1},\y)-1}, 2^{\sigma(E_{x_1},\y)}\right]\]
    holds for any $\vec{y} \in \dom(\y)$ with $\degg^{\I^i}_{E_{x_1}}(\y,\vec{y}) >0$. In the subsequent partitions on $\I'$, we claim that for each $\vec{y} \in \dom(x_1)$, the set of tuples with the same value $\vec{y} \in \dom(x_1)$ always appear together. Suppose {\sc PartitionByAttr}$(\I', x_\ell)$ is invoked with any $\ell \ge 2$. Observe that for any $t \in R^i_j$ with $\pi_{\y_1} t = \vec{y}$, $\pi_{\y_\ell} t = \pi_{\y_\ell} \vec{y}$ always holds since $\y_\ell \subseteq \y_1$, where $\y_1 = \{x_2, x_3, \cdots, x_k\}$ and $\y_\ell = \{x_{\ell+1}, x_{\ell+2}, \cdots, x_k\}$. By line 9 in Algorithm~\ref{alg:partition-hierarchical}, tuples with the same value $\vec{y} \in \dom(x_1)$ always falls into the same sub-relation. In other words, $\degg_{E_{x_1}}(\y_1, \vec{y})$ remains the same in subsequent partitions, for any $\vec{y}$ with $\degg_{E_{x_1}}(\y_1, \vec{y}) >0$. This argument can also generalized to any attribute $x$.
    
    Now, let's interpret the partition process as a directed tree, such that $\I'$ has sub-instances in $\textsc{PartitionByAttr}(\I',x)$ as its children. Each sub-instance returned by Algorithm~\ref{alg:uniformize-hierarchical} corresponds to a distinct root-to-leaf path in this directed tree. Consider an  arbitrary sub-instance $\I''$ corresponding to the root-to-leaf path $\langle \I_1(=\I), \I_2, \cdots, \I_{|\x|} (=\I'')\rangle$. When each instance goes through an invocation of \textsc{PartitionByAttr}$(\I_j, x)$, a distinct value $\sigma(E_x, \y)$ is set up for each of $\I_j$'s children. As proved above, this degree value will be preserved in any $\I_k$ for $k \ge j$. As each instance on this path corresponds to one invocation of \textsc{PartitionByAttr} on a distinct attribute, all possible values of $\sigma(\cdot,\cdot)$ will be set up well for $\I''$. Thus, each sub-instance returned by Algorithm~\ref{alg:uniformize-hierarchical} corresponds to a degree characterization. 
    
    Moreover, for any pair of sub-instances returned by Algorithm~\ref{alg:uniformize-hierarchical}, we can find the lowest common ancestor of these two corresponding root-to-leaf paths, say with an invocation of \textsc{PartitionByAttr} on $x$. So, these two sub-instances must have different degree values over attributes $\y = \{y\in \x: E_x \subsetneq E_y\}$ in relations from $E_x$. As proved above, the difference will be preserved in these two sub-instances.  This argument can be applied to any pair of sub-instances returned by Algorithm~\ref{alg:uniformize-hierarchical}, thus each sub-instances corresponds to a distinct degree characterization.
\end{proof}

In an attribute tree $\T$ rooted at $r$, let $\textsf{path}(r,x)$ be the sequence of attributes lying on the path from $r$ to $x$.

\begin{proof}[Proof of Lemma~\ref{lem:hierarchical-degree-function}]
   We will prove it through the following four steps:
   \begin{itemize}[leftmargin=*]
        \item {\bf Step 1:} $\y' = \{x \in \x: \exists i \in E', j \notin E', x \in \x_i \cap \x_j\}$;
        \item {\bf Step 2:} $\y' \subsetneq (\cap_{i\in E'}\x_i)$;
        \item {\bf Step 3:} there exists no $j \notin E'$ such that $(\cap_{i \in E'} \x_i) \subseteq \x_j$.
        \item {\bf Step 4:} If $x$ is the node such that $\cap_{i \in E'} \x_i = \textsf{path}(r,x)$, let $x' \in \textsf{path}(r,x)$ be the lowest ancestor of $x$ with more than one child. Then, $E' = E_x$ and $\y' = \textsf{path}(r,x')$.    
    \end{itemize}
    
   {\bf Step 1.} It suffices to show that the first property holds for every invocation of $T_{E,\y}$. First, it holds trivially for $T_{E,\partial E}$, which follows the definition of partial attributes $\partial E$. By hypothesis, we assume it holds for some $T_{E, \y}$. Next, we show that it is also preserved in these two recursive rules applied to $T_{E,\y}$. We distinguish two cases.
    \begin{itemize}[leftmargin=*]
        \item $\bar{H}_E$ is disconnected. Consider an arbitrary  connected component $E'' \in \mathcal{C}_E$. For any pair of $i \in E''$ and $j \notin E$, $\x_i \cap \x_j \in \y$ is implied by the hypothesis. For any pair of $i \in E''$ and $j \in E- E''$, $\x_i \cap \x_j \in \y$ is implied by the disconnect fact of $\bar{H}_E$. Together, for any pair of $i \in E''$ and $j \notin E''$, we have $\x_i \cap \x_j \in \y$. Hence, for each $E'' \in \mathcal{C}_E$, $T_{E'', \y \cap (\cup_{i\in E''} \x_i)}$ also satisfies this property.
        \item $\bar{H}_E$ is connected. We note that every attribute in $\cup_{i\in E} \x_i - \y$ only appears in relations from $E$ by hypothesis. As $\y \subseteq (\cap_{i\in E}\x_i)$, every attribute in $\cup_{i\in E}\x_i - (\cap_{i\in E}\x_i)$ only appears in relations from $E$. In other words, if there exists a pair $i \in E$ and $j \notin E$, $\x_i \cap \x_j \in (\cap_{i\in E}\x_i)$. Hence, $T_{E,(\cap_{i\in E}\x_i)}$ also satisfies this property. 
    \end{itemize}
    
    {\bf Step 2.} With the first property, we next prove the second property. From Definition~\ref{def:degree-function}, $\y \subseteq (\cap_{i\in E}\x_i)$. In the base case when $\degg_E(\y,\cdot)$ is invoked, we must have $\y \neq \x_i$, thus $\y \subsetneq \x_i$. In the recursive step when $\bar{H}_E$ is connected, we already show $\y \subsetneq (\cap_{i\in E}\x_i)$. Overall, when $\degg_E(\y,\cdot)$ is invoked, we must have $\y \subsetneq (\cap_{i\in E}\x_i)$.
    
    {\bf Step 3.} Then, we come to the third property. Suppose there exist some $j \in E$ such that $(\cap_{i \in E} \x_i) \subseteq \x_j$. Implied by the first property, $(\cap_{i \in E} \x_i) \subseteq \y$, coming to a contradiction of the second property. 
    
    {\bf Step 4.} Finally, we come to the last step. As $H$ is hierarchical, any subset of relations from $E \subseteq [m]$ also forms a hierarchical join. Attributes in $\cap_{i \in E} \x_i$ form a root-to-node path in the attribute forest of $H$. Together with the third property, if $\textsf{path}(r,x)$ equals to the intersection of relations in $E'$, then $E' = E_x$. 
    Moreover, we note that $\y'$ is also a root-to-node sub-path of $\textsf{path}(r,x)$. Suppose $x' \notin \y'$. Then, we can always find $j \in [m] - E_x$, since $x'$ has at least one child which is not an ancestor of $x$. As $E' = E_x$, we have $j \notin E'$. By definition, $\x' \in \y'$, coming to a contradiction. Under the assumption that every non-leaf attribute in $\mathcal{T}$ has at least two children, it is safe to replace $x'$ with the parent of $x$.
\end{proof}

\begin{proof}[Proof of Lemma~\ref{lem:partition-hierarchical-DP}]
    Consider two neighboring instances $\I$ and $\I'$. Note that $|\degg^\I_{E}(\y, \vec{y}) - \degg^{\I'}_{E}(\y,\vec{y})| \le 1$ holds for any $E \subseteq [m]$, $\y \subseteq (\cap_{i \in E} \x_i)$, and $\vec{y} \in \dom(\y)$. This is not hard to show since change one tuple can change at most one tuple in $\Join_{i \in E} R_i$ as well as one tuple in its projection onto attributes $\cap_{i \in [E]} \x_i$, thus at most one tuple in $\left\{t \in \pi_{\cap_{i \in [E]} \x_i}\Join_{i \in E} R_i: \pi_\y t = \Vec{y} \right\}$. Let $\langle x_1,x_2,\cdots, x_k(=r)\rangle$ be the root-to-leaf path corresponding to $\x_i$. Each input tuple $t \in R_i(\x_i)$ contributes to at most $|\x_i|$ degree functions, i.e., $\degg_{E_{x_i}}(\y, \pi_\y t)$ with $\y = \{x_1,x_2,\cdots,x_{j-1}\}$, for any $j \in [k]$. Hence, $\deg\sim_{(c'\cdot \epsilon, c'\cdot\delta)} \deg'$, where $c' = \max_{i\in[m]} |\x_i|$ is a query-dependent quantity.
    
    Moreover, for each sub-instance $\I^\sigma$ returned, $\F^{\sigma} \sim_{(3\epsilon, 3\delta)} \F'^{\sigma}$ implied by Lemma~\ref{lem:two-table-DP}.
    As each tuple participates in at most $O(\log^c (\frac{n}{\lambda} + 1))$ sub-instances,  $\bigcup_{\sigma} \F^{\sigma} \sim_{(3\log^c (\frac{n}{\lambda} + 1) \cdot \epsilon, 3 \log^c (\frac{n}{\lambda} + 1) \cdot \delta)} \bigcup_{\sigma} \F'^{\sigma}$ implied by the group privacy. Putting everything together, we conclude that Algorithm~\ref{alg:uniformization} preserves $(O(\log^c n \cdot \epsilon), O(\log^c n \cdot \delta))$-DP implied by the sequential composition rule.
\end{proof}

Note that for arbitrary $T_E$, adding noisy degree can only enlarge it by a factor of $\sqrt{2}^{|\x|}$. Let $\y \subseteq \x$ be the set of join attributes, and $\pi_{\y} J = \{t_1, t_2, \cdots, t_k\}$.  We consider the most fine-grained partition of $J$ such that $J_1, J_2, \cdots, J_k$, where $J_i$ corresponds to the set of all join results participated by $t_i \in \dom(\y)$. Let $\pi(i)$ be the degree characterization where $J_i$ falls into with true degrees, and $\widetilde{\pi}(i)$ be the degree characterization where $J_i$ falls into with noisy degrees by Algorithm~\ref{alg:partition-hierarchical}. The cost of Algorithm~\ref{alg:uniformization-framework} on hierarchical joins is 
\begin{align*}
    & \sum_{\sigma} \sqrt{\sum_{\widetilde{\pi}(i) = \sigma}|J_i|} \cdot \sqrt{SS^\sigma_\countsize} \\
   = & \sum_{\sigma} \sqrt{\sum_{i: \pi(i) =\widetilde{\pi}(i) = \sigma}|J_i| + \sum_{i: \pi(i)\neq \sigma, \widetilde{\pi}(i) = \sigma}|J_i|} \cdot \sqrt{SS^\sigma_\countsize} \\
   \le & \sum_{\sigma} \sqrt{\sum_{i: \pi(i) =\widetilde{\pi}(i) = \sigma}|J_i|} \cdot \sqrt{SS^\sigma_\countsize} + \sum_\sigma \sqrt{ \sum_{i: \pi(i)\neq \sigma, \widetilde{\pi}(i) = \sigma}|J_i|} \cdot \sqrt{SS^\sigma_\countsize} \\
   \le & \sum_{\sigma} \sqrt{\sum_{i: \pi(i) =\widetilde{\pi}(i) = \sigma}|J_i|} \cdot \sqrt{SS^\sigma_\countsize} \\
   + & \sum_{\sigma} \sum_{\sigma': \sigma' \neq \sigma} \sqrt{\sum_{i: \pi(i) = \sigma', \widetilde{\pi}(i) = \sigma} |J_i|} \cdot \sqrt{SS^{\sigma'}_\countsize} \cdot \sqrt{2}^{|x|}\\
   =& \sum_\sigma \left(\sqrt{\sum_{i:\pi(i) =\widetilde{\pi}(i) = \sigma} |J_i|} + \sum_{\sigma': \sigma' \neq \sigma} \sqrt{\sum_{i:\pi(i) =\sigma, \widetilde{\pi}(i) = \sigma'} |J_i|} \right) \cdot \sqrt{SS^{\sigma'}_\countsize} \\
   \le & \sum_{\sigma} \sqrt{\sum_{i: \pi(i) = \sigma}|J_i|} \cdot \sqrt{SS^\sigma_\countsize} \cdot \frac{1}{2^{|\x|}}
\end{align*}
where the last inequality is implied by the fact that for any $\sigma$, the number of $\sigma'$ such that some $J_i$ could have $\pi(i) = \sigma$ and $\pi(i) = \sigma'$ is at most $O(2^{|\x|})$.


\begin{proof}[Proof of Theorem~\ref{the:lb-hierarhical-uniformize}]
Let $\mathbb{I}(\OUT_\sigma, \sigma)$ be the set of two-table instances with output size $\OUT_\sigma$ and following the degree characterization $\sigma$. Our proof consists of two steps: 
    \begin{itemize}[leftmargin=*]
        \item {\bf Step (1):} There exists a family of queries $\Q_\sigma$ such that any $(\epsilon,\delta)$-algorithm that takes as input an instance from $\mathbb{I}(\OUT_\sigma, \sigma)$ and outputs an approximate answer to each query in $\Q_\sigma$ within error $\alpha^{\sigma}$ must require $\displaystyle{\alpha^\sigma \ge \Omega\left(\sqrt{\OUT_\sigma} \cdot\sqrt{SS^\sigma_\countsize}\right)}$.
        \item {\bf Step (2):} There exists a family of queries $\Q$ such that any $(\epsilon,\delta)$-algorithm that takes as input an instance $\I(\overrightarrow{\OUT})$ and outputs an approximate answer to each query in $\Q$ within error $\alpha$ must require
        $\displaystyle{\alpha \ge \Omega\left(\max_\sigma \sqrt{\OUT_\sigma} \cdot \sqrt{SS^\sigma_\countsize}\right)}$.
    \end{itemize}
    
    Let's first focus on {\bf step (1)} with arbitrary $\sigma$. Assume $LS^\sigma_\countsize$ is achieved on some $i^* \in [m]$, i.e., $LS^\sigma_\countsize = T^\sigma_{[m]-\{i^*\}}$.
    We compute the value of $T^\sigma_{[m]-\{i^*\}}$ and set $n_\sigma = \frac{\OUT_\sigma}{T_{[m]-\{i\}}}$.
    From Theorem~\ref{the:lb-single-table}, let $\Q^\sigma_\textsf{one}$ be the set of hard queries on which any $(\epsilon,\delta)$-differentially private algorithm takes as input any single table $R_\sigma \in (\{0,1\}^d)^{n_\sigma}$, and outputs an approximate answer to each query in $\Q^\sigma_\textsf{one}$ within error $\alpha$ must require $\alpha \ge \widetilde{\Omega}\left(\sqrt{n_\sigma} \cdot (\frac{\sqrt{d} \cdot \log |\Q^\sigma_\textsf{one}|}{\epsilon})^\frac{1}{2}\right)$. For an arbitrary single table $T^\sigma \in (\{0,1\}^d)^{n_\sigma}$, we can construct an instance $\I^\sigma$ as follows:
    \begin{itemize}[leftmargin=*]
        \item Set $\D^\sigma_j = \prod_{x \in \x_j} \dom(x)$ for any $j \in [m]$;
        \item When visiting attributes of $\mathcal{T}$ in a bottom-up way, say $x$, we set $|\dom(x)| = \sigma(E_x,\y)$ where $\y$ is the set of attributes lying on the path from $r$ to $x$'s parent in $\mathcal{T}$;
        \item For the root $r$, set $\displaystyle{|\dom(r)| = \frac{\OUT_\sigma}{\prod_{x \in \x-\{r\}} \dom(x)}}$;
        \item Every relation is a Cartesian product over its own attributes;
        \item For each data record $x \in R_\sigma$, we exclusively pick a tuple $t \in R_{i^*}$ and attach $x$ to it.
    \end{itemize}
    It can be easily checked that $\I \in \mathbb{I}(\OUT_\sigma,\sigma)$, and $|R_{i^*}| = n_\sigma$. From Theorem~\ref{the:lb-single-table}, let $\Q^\sigma_\textsf{hier}$ be the set of all linear queries over $\D^\sigma_1 \times \D^\sigma_2 \times \cdots \times \D^\sigma_m$. For each query $q \in \Q^\sigma_\textsf{one}$, we construct another query $q'=(q_1,q_2,\cdots, q_m) \in \Q^\sigma_\textsf{hier}$ such that:
    \begin{itemize}[leftmargin=*]
        \item $q_i: \D^\sigma_i \to [-1,1]$ such that $q_i(t) = q(x)$ if and only if $x$ is attached to $t$;
        \item $q_j: \D^\sigma_j \to \{+1\}$ for $j \in [m] - \{i^*\}$.
    \end{itemize}
    We borrow the similar argument from Theorem~\ref{the:lb-two-table}, showing that an $(\epsilon, \delta)$-algorithm that takes an instance in $\mathbb{I}(\OUT_\sigma, \sigma)$ and outputs an approximate answer to each query in $\Q^\sigma_\textsf{hier}$ within error $\alpha$, there exists an $(\epsilon, \delta)$-algorithm that takes an arbitrary single table $R_\sigma \in (\{0,1\})^{n_\sigma}$, and outputs an approximate answer to each query in $\Q^\sigma_\textsf{one}$ within error $\alpha^\sigma/LS^\sigma_\countsize$. As $\alpha^\sigma/LS^\sigma_\countsize \ge \sqrt{n_\sigma}$, $\alpha^\sigma \ge \sqrt{\OUT_\sigma} \cdot \sqrt{LS^\sigma_\countsize}$.
    
    \paragraph{Step (2).} From Theorem~\ref{the:lb-single-table}, let $\Q_\textsf{hier}$ be the family of linear queries over $\D_1 \times \D_2 \times \cdots \D_m$, such that $\displaystyle{\Q_\textsf{hier} = \left\{\cup_{i \in [m]} q_i: q_i \in \Q^{\sigma}_\textsf{hier}, \forall \sigma\right\}}$. Consider an arbitrary $(\epsilon, \delta)$-differentially private algorithm $\mathcal{A}$ takes as input in $\mathbb{I}(\overrightarrow{\OUT})$ and outputs an approximate answer to each query in $\Q_\textsf{hier}$ within error $\alpha$. If $\alpha \le \max_\sigma \sqrt{\OUT_\sigma} \cdot \sqrt{LS^\sigma_\countsize}$, there must exist an $(\epsilon, \delta)$-differentially private algorithm that takes an input any instance from $\mathbb{I}(\overrightarrow{\OUT})$ and output an approximate answer to each query in $\Q^\sigma_\textsf{hier}$ for some $\sigma$, contradicting to {\bf Step (1)}.
\end{proof}

%\begin{lemma}
%    Any partition of the hard instance $\I$ of line-3 join query, as illustrated in Figure~\ref{fig:hard-three-table}, leads to an error of $\Omega(n^{3/4})$.
%\end{lemma}
%
%\begin{proof}
%    Let $k$ be the maximum number of partitions such that a single value from $\dom(B)$ or $\dom(C)$ participates. Note that $k$ is also the maximum number of sub-instances participate by one input tuple from $R_1$ or $R_3$. Implied by the group privacy, the error complexity will be enlarged by a factor of $k$. 
%\end{proof}
\paragraph{Uniformize Acyclic Query.} A join query $\mathcal{H}$ is {\em acyclic} if there is a join tree $\mathcal{T}$ such that every node of $\mathcal{T}$ corresponds to a relation, and for every attribute $x \in \x$, the set of nodes containing $x$ forms a connected subtree of $\mathcal{T}$. For general acyclic join query $\mathcal{H}$, we can first fix a join tree $\mathcal{T}$. Let $\mathcal{C}_E$ be the set of connected components of relations in $E$ on $\mathcal{T}$. For each $E' \in \mathcal{C}_E$, we pick an arbitrary relation $R_i$ with $\x_i \cap \partial E \neq \emptyset$ as the root, which is always feasible; otherwise $E'$ itself is a connected component, and $T_{E'} = |\Join_{i \in E'} R_i|$. After picking $R_i$ as the root, we denote $p(j,i)$ for $j \neq i$ as the parent of $R_j$ in $\mathcal{T}$. For completeness, let $p(i,i) = \x_i \cap \partial E$. Then, 
\[T_{E'} \le \prod_{j \in E'} \max_{t \in \dom(\x_j \cap (\x_{p(j,i)} \cup \partial E))} \big|R_j \ltimes t\big|.\]
At last, $T_E = \prod_{E' \in \mathcal{C}_E} T_{E'}$. To apply the uniformization technique, it suffices to partition each relation $R_i$ by the degree of values in attributes $\x_j \cap (\x_{p(j,i)} \cup \partial E)$, for all possible $E \subseteq [m]$ and root $R_i$. 
